# Supplementary material for: Giant Shear Displacement by Light-Induced Raman Force in Bilayer Graphene
Source: arXiv:2204.08060 ancillary file (2022-04-17)
Supplement: Supplementary file 1 [file SM_arxiv.pdf]

# Supplemental Material for "Giant Shear Displacement by Light-Induced Raman Force in Bilayer Graphene"

Habib Rostami*
*Nordita, KTH Royal Institute of Technology and Stockholm University, Hannes Alfvéns väg 12, 10691 Stockholm, Sweden*
(Dated: April 17, 2022)

## CONTENTS

I. Electron coupling to the shear phonons 1
A. Impact of shear displacement on $\gamma_1$ 2
B. Impact of shear displacement on $\gamma_3$ 2
C. Impact of shear phonon displacement on $\gamma_4$ 3
D. One shear phonon's coupling to electrons 3
E. Two shear phonons' coupling to electrons 3
F. Low-energy two-band model 4
G. Photon-electron-phonon couplings 4

II. Circular and Linear Displacive Raman Force 5

III. Raman force calculation 5
A. Calculation of $\bar{\chi}^{\rm triangle}_{abc}(\omega_1,\omega_2)$ 6
B. Calculation of $\bar{\chi}^{\rm bubble-\gamma}_{abc}(\omega_1,\omega_2)$ 7
C. Calculation of $\bar{\chi}^{\rm bubble-\Theta}_{abc}(\omega_1,\omega_2)$ 7

IV. Finite electronic temperature $T_e$ effect 7

References 8

## I. ELECTRON COUPLING TO THE SHEAR PHONONS

We recall the four-band tight-binding model to describe electronic Hamiltonian of electrons in bilayer graphene [1]

$$H_{\mathbf{k}} = \begin{bmatrix} \epsilon_{A_1} & -\gamma_0 f_{\mathbf{k}} & \gamma_4 f_{\mathbf{k}} & -\gamma_3 f^*_{\mathbf{k}} \\ -\gamma_0 f^*_{\mathbf{k}} & \epsilon_{B_1} & \gamma_1 & \gamma_4 f_{\mathbf{k}} \\ \gamma_4 f^*_{\mathbf{k}} & \gamma_1 & \epsilon_{A_2} & -\gamma_0 f_{\mathbf{k}} \\ -\gamma_3 f_{\mathbf{k}} & \gamma_4 f^*_{\mathbf{k}} & -\gamma_0 f^*_{\mathbf{k}} & \epsilon_{B_2} \end{bmatrix}, \tag{1}$$

where the form factor reads

$$f_{\mathbf{k}} = \sum_{\ell=1}^{3} e^{i\mathbf{k}\cdot\boldsymbol{\delta}_\ell} = e^{ia_0k_y} + 2ie^{-a_0k_y/2}\cos(\sqrt{3}a_0k_s/2). \tag{2}$$

The intralayer nearest neighbour vectors are $\boldsymbol{\delta}_1 = a_0(0,1)$, $\boldsymbol{\delta}_2 = a_0(\sqrt{3}/2,-1/2)$, and $\boldsymbol{\delta}_3 = a_0(-\sqrt{3}/2,-1/2)$. Note that $a_0 \approx 0.14$nm is the carbon-carbon bond length. The two valley points ($\tau = \pm$) are at the corner of hexagonal Brillouin zone: $\tau\mathbf{K} = \tau\frac{4\pi}{\sqrt{3}a_0}\hat{\mathbf{x}}$. Low-energy model is obtain by momentum expansion near the valley point: $\mathbf{k} = \tau\mathbf{K}-\mathbf{q}$ for $q \ll K$ which leads $f_{\mathbf{q}} = \frac{3a_0\gamma_0}{2}(q_x - iq_y)$. The electron-phonon coupling is obtained by considering the dependence of hopping parameters on the phonon displacement.

* habib.rostami@su.se

Shear mode vibration only affect inter-layer hopping elements: $\gamma_1$, $\gamma_3$ and $\gamma_4$. In this section, we calculate one and two-phonon couplings to electrons in bilayer graphene in both four- and two-band models. In the main text, we only consider the impact of one-phonon coupling. The contribution of two-phonon coupling on electrons will be discussed elsewhere.

### A. Impact of shear displacement on $\gamma_1$

The shear phonon displacement $Q$ changes the bond length corresponding to $\gamma_1$ inter-layer hopping as shown in Fig. 1b. However, this correction is second order in $Q$:

$$\gamma_1(\ell) = \gamma_1(c) + \frac{\partial \gamma_1}{\partial c}(\ell - c) + \dots \tag{3}$$

where $c$ and $\ell$ stand for the A2-B1 bond length in the pristine and displaced system, respectively. Therefore, we have

$$\frac{\ell - c}{c} \approx \frac{Q^2}{2c^2} \rightarrow \frac{\delta\gamma_1}{\gamma_1} \approx -\beta_1 \frac{Q^2}{2c^2}. \tag{4}$$

We define $\beta_1 = -\partial \ln \gamma_1 / \partial \ln c$. Accordingly, in the leading one-phonon-electron coupling we can neglect the impact of shear displacement on the vertical $\gamma_1$ hoping.

### B. Impact of shear displacement on $\gamma_3$

The shear phonon displacement $Q$ changes the distance of bond corresponding to $\gamma_3$ inter-layer hopping as shown in Fig. 1b. The change in the hopping $\gamma_3$ is shown by $\delta\gamma_3$ which follows

$$\frac{\delta\gamma_3(d_\ell)}{\gamma_3} = \left(\frac{1}{\gamma_3}\frac{\partial \gamma_3}{\partial b}\right)\Delta d_\ell + \frac{1}{2}\left(\frac{1}{\gamma_3}\frac{\partial^2 \gamma_3}{\partial b^2}\right)(\Delta d_\ell)^2 + \dots \tag{5}$$

Note that $\mathbf{d}_\ell = \boldsymbol{\delta}_\ell + c\hat{z}$ correspond to three A1-B2 bond length in the pristine system and $b = |\mathbf{d}_\ell| = \sqrt{c^2 + a_0^2}$. The change in the bond length then follows

$$\Delta d_\ell = |\mathbf{d}_\ell + \mathbf{Q}_A(\mathbf{R}) - \mathbf{Q}_B(\mathbf{R} - \mathbf{d}_\ell)| - |\mathbf{d}_\ell|, \tag{6}$$

in which $\mathbf{Q}_A$ is the displacement of sublattice A in layer 1 and $\mathbf{Q}_B$ is the displacement of sublattice B in layer 2 at lattice point $\mathbf{R}$. We define the shear displacement $\mathbf{Q}$ as follows

$$\mathbf{Q}_A(\mathbf{R}) - \mathbf{Q}_B(\mathbf{R} - \mathbf{d}_\ell) = \sqrt{2}\mathbf{Q}. \tag{7}$$

Therefore, the change in the bond length reads

$$\Delta d_\ell \approx \frac{\sqrt{2}\mathbf{d}_\ell \cdot \mathbf{Q}}{b}. \tag{8}$$

We find the correction $\delta\gamma_3$ up to second order in the shear displacement field $\mathbf{Q}$:

$$\frac{\delta\gamma_3(d_\ell)}{\gamma_3} = -\beta_3 \frac{\sqrt{2}(\boldsymbol{\delta}_\ell \cdot \mathbf{Q})}{b^2} - \kappa_3 \frac{(\boldsymbol{\delta}_\ell \cdot \mathbf{Q})^2}{b^4}, \tag{9}$$

in which we define

$$\beta_3 = -\frac{\partial \ln \gamma_3}{\partial \ln b} \ , \ \kappa_3 = -\frac{b^2}{\gamma_3}\frac{\partial^2 \gamma_3}{\partial b^2}. \tag{10}$$

Accordingly, the correction to the form-factor for the $\gamma_3$ hopping term reads

$$\begin{aligned} \sum_\ell \frac{\delta\gamma_3(d_\ell)}{\gamma_3} e^{i\mathbf{k}\cdot\boldsymbol{\delta}_\ell} &= -\frac{\sqrt{2}\beta_3}{b^2}\mathbf{Q}\cdot\sum_\ell \boldsymbol{\delta}_\ell e^{i\mathbf{k}\cdot\boldsymbol{\delta}_\ell} - \frac{\kappa_3}{b^4}Q_a Q_b \sum_\ell \delta_\ell^a \delta_\ell^b e^{i\mathbf{k}\cdot\boldsymbol{\delta}_\ell} \\ &= -\frac{\sqrt{2}\beta_3}{b^2}Q_a(-i\partial_{k_a})\sum_\ell e^{i\mathbf{k}\cdot\boldsymbol{\delta}_\ell} - \frac{\kappa_3}{b^4}Q_a Q_b(-i\partial_{k_a})(-i\partial_{k_b})\sum_\ell e^{i\mathbf{k}\cdot\boldsymbol{\delta}_\ell} \\ &= -\frac{\sqrt{2}\beta_3}{b^2}Q_a(-i\partial_{k_a})f_{\mathbf{k}} - \frac{\kappa_3}{b^4}Q_a Q_b(-i\partial_{k_a})(-i\partial_{k_b})f_{\mathbf{k}}, \end{aligned} \tag{11}$$

which simplifies as follows

$$\sum_{\ell} \frac{\delta\gamma_3(d_\ell)}{\gamma_3} e^{i\mathbf{k}\cdot\boldsymbol{\delta}_\ell} = -\beta_3 \frac{\sqrt{2}a_0}{b^2} g_a(\mathbf{k}) Q_a - \kappa_3 \frac{a_0^2}{b^4} h_{ab}(\mathbf{k}) Q_a Q_b. \tag{12}$$

and we define

$$g_a(\mathbf{k}) = \frac{1}{a_0}(-i\partial_{k_a}) f_{\mathbf{k}} \quad , \quad h_{ab}(\mathbf{k}) = -\frac{1}{a_0^2}\partial_{k_a}\partial_{k_b} f_{\mathbf{k}} \ . \tag{13}$$

### C. Impact of shear phonon displacement on $\gamma_4$

Similar to the case of $\gamma_3$, one can obtain the correction to $\gamma_4$-related form-factors as follows

$$\sum_{\ell} \frac{\delta\gamma_4(d_\ell)}{\gamma_4} e^{i\mathbf{k}\cdot\boldsymbol{\delta}_\ell} = -\beta_4 \frac{\sqrt{2}a_0}{b^2} g_a(\mathbf{k}) Q_a - \kappa_4 \frac{a_0^2}{b^4} h_{ab}(\mathbf{k}) Q_a Q_b, \tag{14}$$

where

$$\beta_4 = -\frac{\partial \ln \gamma_4}{\partial \ln b} \ , \ \kappa_4 = -\frac{b^2}{\gamma_4}\frac{\partial^2 \gamma_4}{\partial b^2}. \tag{15}$$

### D. One shear phonon's coupling to electrons

In the four-band model, the coupling of one shear phonon to electrons can be written as follows

$$H_{ep} = \sum_{\mathbf{k}} \sum_{a} \hat{\Psi}^\dagger_{\mathbf{k}} \hat{M}_a(\mathbf{k}) \hat{\Psi}_{\mathbf{k}} \hat{Q}_a, \tag{16}$$

where the electron-phonon matrix element is given by

$$\hat{M}_a(\mathbf{k}) = \begin{bmatrix} 0 & 0 & -\alpha_4 g_a(\mathbf{k}) & \alpha_3 g_a^*(\mathbf{k}) \\ 0 & 0 & 0 & -\alpha_4 g_a(\mathbf{k}) \\ -\alpha_4 g_a^*(\mathbf{k}) & 0 & 0 & 0 \\ \alpha_3 g_a(\mathbf{k}) & -\alpha_4 g_a^*(\mathbf{k}) & 0 & 0 \end{bmatrix}, \tag{17}$$

where we define $\alpha_i = (\sqrt{2}\beta_i a_0/b^2)\gamma_i$.

### E. Two shear phonons' coupling to electrons

In the four-band model the coupling of two shear phonons to electrons reads

$$\hat{H}_{ep} = \sum_{\mathbf{k}} \sum_{ab} \hat{\Psi}^\dagger_{\mathbf{k}} \hat{W}_{ab}(\mathbf{k}) \hat{\Psi}_{\mathbf{k}} \hat{Q}_a \hat{Q}_b, \tag{18}$$

where the electron-phonon matrix element is given by

$$\hat{W}_{ab}(\mathbf{k}) = \begin{bmatrix} 0 & 0 & -\eta_4 h_{ab}(\mathbf{k}) & \eta_3 h_{ab}^*(\mathbf{k}) \\ 0 & 0 & -\eta_1 \delta_{ab} & -\eta_4 h_{ab}(\mathbf{k}) \\ -\eta_4 h_{ab}^*(\mathbf{k}) & -\eta_1 \delta_{ab} & 0 & 0 \\ \eta_3 h_{ab}(\mathbf{k}) & -\eta_4 h_{ab}^*(\mathbf{k}) & 0 & 0 \end{bmatrix}, \tag{19}$$

where we define

$$\eta_1 = \frac{\beta_1}{2c^2}\gamma_1 \ , \eta_3 = \frac{\kappa_3 a_0^2}{b^4}\gamma_3 \ , \eta_4 = \frac{\kappa_4 a_0^2}{b^4}\gamma_4 \ . \tag{20}$$

### F. Low-energy two-band model

In this subsection, we obtain a two-band model Hamiltonian for the electron couplings to shear phonons up to second order in electron momentum and phonon displacement field. We follow the effective Green's function approach [2] to drive to effective Hamiltonian. Consider 4×4 Hamiltonian and Green's function written in terms of 2×2 blocks $\hat{H}_{ij}$ and $\hat{G}_{ij}$:

$$\hat{H} = \begin{bmatrix} \hat{H}_{11} & \hat{H}_{12} \\ \hat{H}_{21} & \hat{H}_{22} \end{bmatrix} \quad , \quad \hat{G} = \begin{bmatrix} \hat{G}_{11} & \hat{G}_{12} \\ \hat{G}_{21} & \hat{G}_{22} \end{bmatrix}. \tag{21}$$

Note that the Green's function is defined as $\hat{G}(\hat{E} - \hat{H}) = \hat{I}$. One can simply show

$$\hat{G}_{11}\{E - \hat{H}_{11} - \hat{H}_{12}(E - \hat{H}_{22})^{-1}\hat{H}_{21}\} = \hat{I}. \tag{22}$$

At low energy of gapless system we can set $E = 0$ and we rewrite

$$\hat{G}_{11}\{E - \hat{H}_{11} + \hat{H}_{12}\hat{H}_{22}^{-1}\hat{H}_{21}\} = \hat{G}_{11}(E - \hat{H}_{\text{eff}}) = \hat{I}, \tag{23}$$

where the effective Hamiltonian reads

$$\hat{H}_{\text{eff}} = \hat{H}_{11} - \hat{H}_{12}\hat{H}_{22}^{-1}\hat{H}_{21}. \tag{24}$$

We follow the above steps and obtain the low-energy Hamiltonian

$$\hat{H}_{\text{eff}} = \sum_{\mathbf{k}} \hat{\Psi}_{\mathbf{k}}^{\dagger} \left\{ \hat{H}_{\mathbf{k}} + \sum_{a} \hat{M}_a(\mathbf{k}) Q_a + \sum_{ab} \hat{W}_{ab}(\mathbf{k}) Q_a Q_b \right\} \hat{\Psi}_{\mathbf{k}}. \tag{25}$$

The two-band kinetic Hamiltonian thus reads

$$H_{\mathbf{q}} = -\frac{\hbar^2}{2m} \begin{bmatrix} 0 & (\tau q_x - i q_y)^2 \\ (\tau q_x + i q_y)^2 & 0 \end{bmatrix}, \tag{26}$$

in which the effective mass is related to both intra and inter-layer hopping energies

$$\frac{\hbar^2}{2m} = \frac{9 a_0^2 \gamma_0^2}{4\gamma_1}, \tag{27}$$

The electron-phonon interaction at $\mathbf{q} = \mathbf{0}$ is given by

$$(\hat{M}_x, \hat{M}_y) = \frac{3\alpha_3}{2}(\tau\hat{\sigma}_y, \hat{\sigma}_x). \tag{28}$$

For two-phonon-electron term at $\mathbf{q} = \mathbf{0}$, the only non-vanishing terms are

$$\hat{W} = \begin{bmatrix} \hat{W}_{xx} & \hat{W}_{xy} \\ \hat{W}_{yx} & \hat{W}_{yy} \end{bmatrix} = \frac{3}{2}\left(\frac{3\alpha_4^2}{\gamma_1} - \eta_3\right) \begin{bmatrix} \hat{\sigma}_x & \tau\hat{\sigma}_y \\ \tau\hat{\sigma}_y & -\hat{\sigma}_x \end{bmatrix}. \tag{29}$$

### G. Photon-electron-phonon couplings

In order to calculate the mixed vertex coupling for photon-electron-phonon couplings, we start with minimal transformation $\mathbf{k} \to \mathbf{k} + e\mathbf{A}(t)/\hbar$ in electron-phonon interaction Hamiltonian given in Eq. (30) and Eq. (19). For instance, the photon-electron-phonon vertex coupling is obtained as follows:

$$\begin{aligned} \hat{M}_a(\mathbf{k} + e\mathbf{A}(t)/\hbar) &= \begin{bmatrix} 0 & 0 & -\alpha_4 g_a(\mathbf{k} + e\mathbf{A}(t)/\hbar) & \alpha_3 g_a^*(\mathbf{k} + e\mathbf{A}(t)/\hbar) \\ 0 & 0 & 0 & -\alpha_4 g_a(\mathbf{k} + e\mathbf{A}(t)/\hbar) \\ -\alpha_4 g_a^*(\mathbf{k} + e\mathbf{A}(t)/\hbar) & 0 & 0 & 0 \\ \alpha_3 g_a(\mathbf{k} + e\mathbf{A}(t)/\hbar) & -\alpha_4 g_a^*(\mathbf{k} + e\mathbf{A}(t)/\hbar) & 0 & 0 \end{bmatrix} \\ &\approx \frac{e a_0 A_b(t)}{\hbar} \begin{bmatrix} 0 & 0 & -i\alpha_4 h_{ab}(\mathbf{k}) & -i\alpha_3 h_{ab}^*(\mathbf{k}) \\ 0 & 0 & 0 & -i\alpha_4 h_{ab}(\mathbf{k}) \\ i\alpha_4 h_{ab}^*(\mathbf{k}) & 0 & 0 & 0 \\ i\alpha_3 h_{ab}(\mathbf{k}) & i\alpha_4 h_{ab}^*(\mathbf{k}) & 0 & 0 \end{bmatrix}. \end{aligned} \tag{30}$$

Afterward, we follow the previous section's procedure and obtain a low-energy two-band model for the above photon-mediated electron-phonon interaction. The final result, at leading order in electronic momentum $\mathbf{k}$, is give in Eq. (6). Similar approach can be used to obtain two-phonon-electron coupling mediated by photons starting from $\hat{W}_{ab}(\mathbf{k} + e\mathbf{A}(t)/\hbar)$.

## II. CIRCULAR AND LINEAR DISPLACIVE RAMAN FORCE

The rectification (displaciv) Raman force is obtained by setting $\omega_1 + \omega_2 = 0$. In response to a monochromatic external electric field $\mathbf{E}(t) = 2\mathrm{Re}[\mathbf{E}(\omega)e^{i\omega t}]$, it can be formally written as follows

$$\mathcal{F}^{\mathrm{dc}}_a = \sigma^{\mathrm{R}}_{abc}(\omega,-\omega)E_b(\omega)E^*_c(\omega)\ , \tag{31}$$

where $\sigma^{\mathrm{R}}_{abc}(\omega,-\omega) = \sigma^{\mathrm{R}}_{abc}(-\omega,\omega) = -\chi^{\mathrm{R}}_{abc}(\omega,-\omega)/\omega^2$ is the gauge-invariant displacive Raman response function. The reality of the electric field in the time-domain implies $\mathbf{E}(-\omega) = \mathbf{E}^*(\omega)$. We decompose linear and circular rectification processes by utilizing the following relation

$$\begin{aligned} E_b(\omega)E^*_c(\omega) &= \frac{E_b(\omega)E^*_c(\omega) + E_c(\omega)E^*_b(\omega)}{2} + \frac{E_b(\omega)E^*_c(\omega) - E_c(\omega)E^*_b(\omega)}{2} \\ &= \mathrm{Re}[E_b(\omega)E^*_c(\omega)] + \frac{1}{2}\epsilon_{\ell bc}[\mathbf{E}(\omega)\times\mathbf{E}^*(\omega)]_\ell\ , \end{aligned} \tag{32}$$

where the first and second terms on the right side of the above relation leads the linear and displacive Raman force, respectively. In analogous to linear and circular photgalvanic effect [3], the Raman response function can be decomposed into symmetric and antisymmetric parts standing for the linear and circular displacive force contributions, respectively:

$$\sigma^{\mathrm{R}}_{abc}(\omega,-\omega) = \frac{\sigma^{\mathrm{R}}_{abc}(\omega,-\omega) + \sigma^{\mathrm{R}}_{acb}(\omega,-\omega)}{2} + \frac{\sigma^{\mathrm{R}}_{abc}(\omega,-\omega) - \sigma^{\mathrm{R}}_{acb}(\omega,-\omega)}{2} = \sigma^{\mathrm{LDR}}_{abc}(\omega,-\omega) + \sigma^{\mathrm{CDR}}_{abc}(\omega,-\omega). \tag{33}$$

Note that LDR/CDR indicate the linear/circular displacive Raman force. Considering the electric field in the $xy$-plane and for the case of CDR, we have

$$\mathcal{F}^{\mathrm{CDR}}_\alpha = \gamma^{\mathrm{CDR}}_a(\omega)[i\mathbf{E}(\omega)\times\mathbf{E}^*(\omega)]\cdot\hat{\mathbf{z}}, \tag{34}$$

where the circular displacive Raman response function is given by

$$\gamma^{\mathrm{CDR}}_a(\omega) = \frac{\sigma^{\mathrm{R}}_{axy}(\omega,-\omega) - \sigma^{\mathrm{R}}_{ayx}(\omega,-\omega)}{2i}\ . \tag{35}$$

The intrinsic permutation symmetry [4] implies that $\sigma^{\mathrm{R}}_{\alpha yx}(\omega,-\omega) = \sigma^{\mathrm{R}}_{\alpha xy}(-\omega,\omega)$ and thus we obtain

$$\gamma^{\mathrm{CDR}}_a(\omega) = \frac{\sigma^{\mathrm{R}}_{axy}(\omega,-\omega) - \sigma^{\mathrm{R}}_{axy}(-\omega,\omega)}{2i} = \mathrm{Im}[\sigma^{\mathrm{R}}_{axy}(\omega,-\omega)]\ . \tag{36}$$

Due to the reality of the electric field and the current, we have $\mathbf{E}^*(\omega) = \mathbf{E}(-\omega)$ and $[\sigma^{\mathrm{R}}_{axy}(\omega,-\omega)]^* = \sigma^{\mathrm{R}}_{axy}(-\omega,\omega)$. For the linear displacive Raman force (LDR), we find

$$\mathcal{F}^{\mathrm{LDR}}_a = \gamma^{\mathrm{CDR}}_{abc}(\omega)\mathrm{Re}[E_b(\omega)E^*_c(\omega)]. \tag{37}$$

Using the permutation symmetry and the reality of current and electric field [4], we have $\sigma^{\mathrm{R}}_{acb}(\omega,-\omega) = \sigma^{\mathrm{R}}_{abc}(-\omega,\omega) = [\sigma^{\mathrm{R}}_{abc}(\omega,-\omega)]^*$. Therefore, we obtain

$$\gamma^{\mathrm{LDR}}_{abc}(\omega) = \frac{\sigma^{\mathrm{R}}_{abc}(\omega,-\omega) + \sigma^{\mathrm{R}}_{acb}(\omega,-\omega)}{2} = \mathrm{Re}[\sigma^{\mathrm{R}}_{abc}(\omega,-\omega)]. \tag{38}$$

## III. RAMAN FORCE CALCULATION

Here, we provide details of calculations for the Feynman diagrams given in Fig. 2. The total Raman response function is obtained as follows

$$\chi^{\mathrm{R}}_{abc}(\omega_1,\omega_2) = \chi^{\mathrm{triangle}}_{abc}(\omega_1,\omega_2) + \chi^{\mathrm{bubble}-\gamma}_{abc}(\omega_1,\omega_2) + \chi^{\mathrm{bubble}-\Theta}_{abc}(\omega_1,\omega_2) + \chi^{\mathrm{bubble}-\Delta}_{abc}. \tag{39}$$

The contribution of 2photon-electron-phonon coupling $\Delta_{abc}$ depicted in diagram in Fig. 2d is frequency independent and therefore it can be fixed by enforcing the gauge invariance that implies a response to the static homogeneous

gauge field must vanish due to the gauge invariance, i.e. $\chi^{\rm R}_{abc}(\omega_1 = 0, \omega_2 = 0) = 0$. Since gauge invariance demands $\chi^{\rm R}_{abc}(\omega_1 = 0, \omega_2 = 0) = 0$, we have

$$\chi^{\rm bubble-\Delta}_{abc} = -\chi^{\rm triangle}_{abc}(0,0) - \chi^{\rm bubble-\gamma}_{abc}(0,0) - \chi^{\rm bubble-\Theta}_{abc}(0,0). \tag{40}$$

Therefore, we find

$$\chi^{\rm R}_{abc}(\omega_1,\omega_2) = \bar{\chi}^{\rm triangle}_{abc}(\omega_1,\omega_2) + \bar{\chi}^{\rm bubble-\gamma}_{abc}(\omega_1,\omega_2) + \bar{\chi}^{\rm bubble-\Theta}_{abc}(\omega_1,\omega_2). \tag{41}$$

in which we define $\bar{\chi}_{abc}(\omega_1,\omega_2) = \chi_{abc}(\omega_1,\omega_2) - \chi_{abc}(0,0)$. In the following, we explicitly calculate these three remaining diagrams using low-energy two-band model of bilayer graphene given in Eq. (5) and electron-phonon couplings Eq. (6).

### A. Calculation of $\bar{\chi}^{\rm triangle}_{abc}(\omega_1,\omega_2)$

The triangle diagram Fig. 2a can be written in terms of electronic Green's function $\hat{G}(\mathbf{k}, ik_n)$ and electron-phonon matrix-element $\hat{M}_a$ and paramagnetic current operator $\hat{j}_b, \hat{j}_c$:

$$\chi_{abc}(i\omega_{m_1}, i\omega_{m_2}) = \frac{1}{S}\sum_{\mathbf{k}}\frac{1}{\beta}\sum_{ik_n}{\rm Tr}\left[\hat{M}_a(\mathbf{k})\hat{G}(\mathbf{k},ik_n)\hat{j}_b(\mathbf{k})\hat{G}(\mathbf{k},ik_n+i\omega_{m_1})\hat{j}_c(\mathbf{k})\hat{G}(\mathbf{k},ik_n+i\omega_{m_1}+i\omega_{m_2})\right]. \tag{42}$$

where the trace operator Tr[...] sum over all spinor degree of freedom, $\beta = 1/k_{\rm B}T_e$, $ik_n$ ($i\omega_m$) stands for the femionic (bosonic) Matsubara frequency. From now on, we adopt a short-hand notation $ik_n \to n$ and $i\omega_m \to m$ for the sake of simplicity. The electronic Green's function is given as follows

$$\hat{G}(\mathbf{k}, ik_n) = [ik_n - \hat{H}_{\mathbf{k}}]^{-1}. \tag{43}$$

Because of the mirror symmetry $x \to -x$ the response tensor elements with odd Cartesian index $x$ vanishes $\chi_{xxx} = \chi_{yxy} = \chi_{xyy} = \chi_{yyx} = 0$. This symmetry consideration is confirmed by an explicit calculation based on the low-energy two-band model. The remaining tensor elements also related to each other due to the rotation symmetry of the system:

$$\chi_{yyy} = \chi_{xxy} = \chi_{xyx} = -\chi_{yxx} = \chi_1. \tag{44}$$

After performing the integration on the azimuthal angle of electronic wave vector $\mathbf{k}$ and using the low-energy dispersion $\epsilon_{\mathbf{k}} = \hbar^2k^2/2m$ and $kdk = (m/\hbar^2)d\epsilon$ we find

$$\chi_1(m_1,m_2) = \left(\frac{N_fM}{2\pi}\right)\left(\frac{e}{m}\right)^2\left(\frac{m}{\hbar^2}\right)\int_0^\infty d\epsilon\frac{1}{\beta}\sum_n\frac{8\epsilon^2\xi(n)\xi(m_1+m_2+n)}{(\epsilon^2-\xi(n)^2)(\epsilon^2-\xi(m_1+n)^2)(\epsilon^2-\xi(m_1+m_2+n)^2)}. \tag{45}$$

where $\xi(n) = \mu + n$. After performing Matsubara summation and integrating over $\epsilon$ at zero temperature, we find

$$\chi_1(\omega_1,\omega_2) = \frac{N_fMe^2}{8\pi\hbar^2}\Big\{A_1\ln[4\epsilon^2-\omega_1^2] + A_2\ln[4\epsilon^2-\omega_2^2] + A_3\ln[4\epsilon^2-(\omega_1+\omega_2)^2]\Big\}_{\epsilon\to\mu}^{\epsilon\to\infty}. \tag{46}$$

where

$$A_1 = \frac{\omega_1(\omega_1+2\omega_2)}{\omega_2(\omega_1+\omega_2)}\ ,\quad A_2 = \frac{\omega_2(\omega_2+2\omega_1)}{\omega_1(\omega_1+\omega_2)}\ ,\quad A_3 = -\frac{(\omega_1+2\omega_2)^2}{\omega_2\omega_2} = -1-(A_1+A_2). \tag{47}$$

By subtracting the zero-frequency contribution and after some simplifications, we find

$$\chi_1(\omega_1,\omega_2) - \chi_1(0,0) = \frac{N_fMe^2}{8\pi\hbar^2}\left\{A_1\ln\left[\frac{4\epsilon^2-\omega_1^2}{4\epsilon^2-(\omega_1+\omega_2)^2}\right] + A_2\ln\left[\frac{4\epsilon^2-\omega_2^2}{4\epsilon^2-(\omega_1+\omega_2)^2}\right] - \ln\left[\frac{4\epsilon^2-(\omega_1+\omega_2)^2}{4\epsilon^2}\right]\right\}_{\epsilon\to\mu}^{\epsilon\to\infty}. \tag{48}$$

Eventually, we obtain $\bar{\chi}^{\rm triangle}_{yyy}(\omega_1,\omega_2) = \chi_1(\omega_1,\omega_2) - \chi_1(0,0)$ as follows

$$\bar{\chi}^{\rm triangle}_{yyy}(\omega_1,\omega_2) = \frac{N_fMe^2}{8\pi\hbar^2}\left\{\ln\left[1-\frac{(\omega_1+\omega_2)^2}{4\mu^2}\right] - A_1\ln\left[\frac{4\mu^2-\omega_1^2}{4\mu^2-(\omega_1+\omega_2)^2}\right] - A_2\ln\left[\frac{4\mu^2-\omega_2^2}{4\mu^2-(\omega_1+\omega_2)^2}\right]\right\}. \tag{49}$$

### B. Calculation of $\bar{\chi}^{\rm bubble-\gamma}_{abc}(\omega_1,\omega_2)$

The bubble diagram Fig. 2b can be written in terms of electronic Green's function $\hat{G}(\mathbf{k},n)$, electron-phonon matrix-element $\hat{M}_a$ and the Raman vertex $\hat{\gamma}_{bc}$:

$$\chi_{abc}(m_1,m_2) = -\frac{1}{S}\sum_{\mathbf{k}}\frac{1}{\beta}\sum_n {\rm Tr}\left[\hat{\mathcal{M}}^{(1)}_a \hat{G}(\mathbf{k},n)\hat{\gamma}_{bc}\hat{G}(\mathbf{k},n+m_1+m_2)\right]. \tag{50}$$

The over-all minus sign originates from the standard rules of Feynman diagrams [5], also see [6]. Similar to the previous diagram, we have $\chi_{xxx} = \chi_{yxy} = \chi_{xyy} = \chi_{yyx} = 0$ by symmetry. The other non-vanishing tensor elements read

$$\chi_{yyy} = \chi_{xxy} = \chi_{xyx} = -\chi_{yxx} = \chi_2. \tag{51}$$

After performing the integration on the azimuthal angle of electronic wave vector $\mathbf{k}$ and using the low-energy dispersion $\epsilon_{\mathbf{k}} = \hbar^2k^2/2m$ and $kdk = (m/\hbar^2)d\epsilon$ we find

$$\chi_2(m_1,m_2) = N_f\frac{m}{\hbar^2}\frac{e^2M}{2\pi m}\int_0^\infty d\epsilon\frac{1}{\beta}\sum_n\frac{2\xi(n)\xi(m_1+m_2+n)}{(\epsilon^2-\xi(n)^2)\,(\epsilon^2-\xi(m_1+m_2+n)^2)}. \tag{52}$$

After performing the summation on the Matsubara frequency $n$ and subtracting the zero-frequency contribution we find

$$\chi_2(\omega_1,\omega_2)-\chi_2(0,0) = -\frac{N_fMe^2}{8\pi\hbar^2}\Big\{\ln[\frac{4\epsilon^2-(\omega_1+\omega_2)^2}{4\epsilon^2}]\Big\}^{\epsilon\to\infty}_{\epsilon\to\mu}. \tag{53}$$

Finally, we obtain

$$\chi^{\rm bubble-\gamma}_{yyy}(\omega_1,\omega_2) = -\frac{N_fMe^2}{8\pi\hbar^2}\ln\left[1-\frac{(\omega_1+\omega_2)^2}{4\mu^2}\right]. \tag{54}$$

### C. Calculation of $\bar{\chi}^{\rm bubble-\Theta}_{abc}(\omega_1,\omega_2)$

The bubble diagram Fig. 2c can be written in terms of electronic Green's function $\hat{G}(\mathbf{k},n)$, 1photon-electron-phonon vertex $\hat{\Theta}_{ab}$ and the paramagnetic current $\hat{j}_c$. Considering the permutation symmetry, we have

$$\begin{aligned}\chi_{abc}(m_1,m_2) = &-\frac{1}{2S}\sum_{\mathbf{k}}\frac{1}{\beta}\sum_n {\rm Tr}\left[\hat{\Theta}_{ab}\hat{G}(\mathbf{k},n)\hat{j}_c(\mathbf{k})\hat{G}(\mathbf{k},n+m_2)\right]\\ &-\frac{1}{2S}\sum_{\mathbf{k}}\frac{1}{\beta}\sum_n {\rm Tr}\left[\hat{\Theta}_{ac}\hat{G}(\mathbf{k},n)\hat{j}_b(\mathbf{k})\hat{G}(\mathbf{k},n+m_1)\right].\end{aligned} \tag{55}$$

Using the isotropic approximation for the photon-electron-phonon vertex given in Eq. (6) and after performing the integration on the azimuthal angle of electronic wave vector $\mathbf{k}$, we obtain a vanishing result for all tensor elements. Therefore, within our low-energy model analysis, the mix photon-electron-phonon coupling does not contribute to the Raman force:

$$\bar{\chi}^{\rm bubble-\Theta}_{abc}(\omega_1,\omega_2) = 0. \tag{56}$$

## IV. FINITE ELECTRONIC TEMPERATURE $T_e$ EFFECT

At finite electronic temperature, we first need to calculate the temperature dependence of the chemical potential. Using the isotropic two-band model of bilayer graphene we can easily show that chemical potential is equal to the Fermi energy: $\mu = \epsilon_{\rm F}$ [7]. I summarise this derivation as follows: The total charge density is given in terms of electron and hole density $-en = -e|n_e - n_h|$ where

$$n = \frac{N_f}{S}\sum_p(n_{\rm F}(\epsilon_p)+n_{\rm F}(-\epsilon_p)-1) = \frac{N_fmk_{\rm B}T_e}{2\pi\hbar^2}\int_0^\infty dx\left\{\frac{1}{1+e^{x-\frac{\mu}{k_{\rm B}T_e}}}-\frac{1}{1+e^{x+\frac{\mu}{k_{\rm B}T_e}}}\right\} = \frac{2m\epsilon_F}{\pi\hbar^2}. \tag{57}$$

Note that we have used $\epsilon_p = p^2/2m$. We can simplify the above relation as follows

$$\frac{\epsilon_F}{k_B T_e} = \int_0^\infty dx \left\{ \frac{1}{1+e^{x-\frac{\mu}{k_B T_e}}} - \frac{1}{1+e^{x+\frac{\mu}{k_B T_e}}} \right\}, \tag{58}$$

and thus we find

$$\frac{\epsilon_F}{k_B T_e} = \ln[1+e^{\frac{\mu}{k_B T_e}}] - \ln[1+e^{\frac{-\mu}{k_B T_e}}]. \tag{59}$$

One can quickly solve the above relation and find $\mu = \epsilon_F$. For finite electronic temperature $T_e$, we can utilise the following identity [8]

$$\frac{1}{e^x+1} = \int_{-\infty}^{\infty} \frac{\Theta(y-x)}{4\cosh^2(y/2)} dy, \tag{60}$$

where $\Theta(x)$ is the Heaviside step function. Using the above identity, we calculate finite temperature response function by integrating over the zero temperature one. Accordingly, we replace $\ell_n(z,\mu) = |\mu|^n \ln[(z-2|\mu|)/(z+2|\mu|)]$ with $L_n(z,\mu,T)$ and we numerically solve the integration:

$$L_n(z,\mu,T_e) = \int_{-\infty}^{+\infty} dx \frac{\ell_n(z,x)}{4k_B T_e \cosh^2(\frac{x-\mu}{2k_B T_e})}. \tag{61}$$


[1] E. McCann and M. Koshino, Reports on Progress in Physics **76**, 056503 (2013).
[2] E. McCann and V. I. Fal'ko, Phys. Rev. Lett. **96**, 086805 (2006).
[3] V. I. Belinicher and B. I. Sturman, Soviet Physics Uspekhi **23**, 199 (1980).
[4] P. Butcher and D. Cotter, *The Elements of Nonlinear Optics, Cambridge Univ* (Press, Cambridge, 1990).
[5] G. D. Mahan, *Many-particle physics* (Springer US, 1995).
[6] H. Rostami, M. I. Katsnelson, G. Vignale, and M. Polini, Annals of Physics **431**, 168523 (2021).
[7] S. Adam and M. D. Stiles, Phys. Rev. B **82**, 075423 (2010).
[8] G. Giuliani and G. Vignale, *Quantum theory of the electron liquid* (Cambridge university press, 2005).
